# Supplementary material for: Intensity-dependent precision two-photon Doppler-free spectroscopy of Xe using narrow-bandwidth long-pulse deep-UV laser radiation
Source: arXiv:2509.08136 source file (2025-09-09)
Supplement: Supplementary file 1 [file Supplemental_Material.pdf]

# Supplemental Material for “Intensity-dependent precision two-photon Doppler-free spectroscopy of Xe using narrow-bandwidth long-pulse deep-UV laser radiation”

M. H. Rayment, R. Stech, and F. Merkt

*Institute for Molecular Physical Science, ETH Zürich, 8093 Zürich, Switzerland*

(Dated: September 9, 2025)

This supplemental material presents, in Tables I to VI, the auxiliary data used to determine the relative positions of the  $6s[3/2]_2$ ,  $6s'[1/2]_0$ ,  $6p[1/2]_0$ ,  $8s[3/2]_1$  and  $8d[1/2]_1$  low-lying electronic states of  $^{136}\text{Xe}$  using different combinations of reference IR transition frequencies from Ref. [S1, S2]. The supplemental material also presents, in Table SVII, the auxiliary data from Refs. [S3–S8] used to determine these isotopic shifts from isotopic-shift measurements of transitions between low-lying electronic states of Xe.

These relative positions and isotopic shifts are used in the main article to clarify a discrepancy of about 1 GHz between values of the first ionization energy of Xe obtained by extrapolation of the  $[\text{Xe}^+ (5p)^5 \ ^2P_{3/2}]np/f \leftarrow (5p)^5(6s)[3/2]_2$  Rydberg series in Ref. [S9] and of the  $[\text{Xe}^+ (5p)^5 \ ^2P_{3/2}]np/f \leftarrow (5p)^5(6s')[1/2]_0$  Rydberg series in Ref. [S10]. The same IR-spectroscopic data are also used, in the main article, to obtain improved values of the first ionization energy of  $^{136}\text{Xe}$  and of natural Xe in an analysis that also includes precision measurements of Xe transitions and isotopic shifts in the UV and VUV ranges of the electromagnetic spectrum from Refs. [S8, S9, S11–S13].

The analysis involved checking the consistency of spectroscopic data sets in different spectral ranges obtained with different methods and, in some cases, estimating the uncertainties of relative and absolute experimental frequencies. For instance, the data reported by Humphreys and Paul [S1], which represents the most extensive set of IR transition wavenumbers in Xe, do not include uncertainties. We estimated them to be  $0.001 \text{ cm}^{-1}$  by comparing with results reported by Littlefield and Rafi [S2], who remeasured several of the transitions studied by Humphreys and Paul using the same experimental approach and who carried out repeated measurements of the same transitions. Several of the most precise investigations of isotopic shifts did not report absolute frequencies [S3–S8], but only frequency differences. The corresponding data could therefore only be used to determine isotopically weighted quantities for comparison with frequencies reported for natural Xe without specification of the isotopes.

TABLE I. Determination of the  $8s [3/2]_1$  to  $6p [1/2]_0$  wavenumber interval (in  $\text{cm}^{-1}$ ) for the  $^{136}\text{Xe}$  isotope. The first column indicates the sequence of measured transitions used to connect these two states and the arrows point away from (towards) the lower-lying (higher-lying) energy level. The references in the third column give the sources of the data used in the same order as in the first column (see text for details).

| Connection from $8s [3/2]_1$ to $6p [1/2]_0$ state                                                                           | $(E_{6p [1/2]_0} - E_{8s [3/2]_1})/hc$ | Data origin              |
|------------------------------------------------------------------------------------------------------------------------------|----------------------------------------|--------------------------|
| $8s [3/2]_1 \leftarrow 6p [5/2]_2 \rightarrow 6d [3/2]_1 \leftarrow 6p [1/2]_0$                                              | -10813.4725(17)                        | [S1] [S1] [S1]           |
| $8s [3/2]_1 \leftarrow 6p [3/2]_2 \rightarrow 7d [1/2]_1 \leftarrow 6p [1/2]_0$                                              | -10813.4729(17)                        | [S1] [S1] [S1]           |
| $8s [3/2]_1 \leftarrow 6p [1/2]_1 \rightarrow 7d [1/2]_1 \leftarrow 6p [1/2]_0$                                              | -10813.4725(17)                        | [S1] [S1] [S1]           |
| $8s [3/2]_1 \leftarrow 6p [1/2]_1 \rightarrow 6d [3/2]_1 \leftarrow 6p [1/2]_0$                                              | -10813.4729(17)                        | [S1] [S1] [S1]           |
| $8s [3/2]_1 \leftarrow 6p [1/2]_1 \rightarrow 7d [3/2]_1 \leftarrow 6p [1/2]_0$                                              | -10813.4722(17)                        | [S1] [S1] [S1]           |
| $8s [3/2]_1 \leftarrow 6p [5/2]_2 \leftarrow 6s [3/2]_2 \rightarrow 6p [3/2]_1 \rightarrow 5d [3/2]_1 \leftarrow 6p [1/2]_0$ | -10813.4719(22)                        | [S1] [S1] [S1] [S1] [S1] |
|                                                                                                                              | -10813.4725(23)                        | [S1] [S2] [S1] [S1] [S1] |
|                                                                                                                              | -10813.4715(26)                        | [S1] [S1] [S2] [S1] [S1] |
|                                                                                                                              | -10813.4721(26)                        | [S1] [S2] [S2] [S1] [S1] |
|                                                                                                                              | -10813.4715(20)                        | [S1] [S1] [S1] [S1] [S2] |
|                                                                                                                              | -10813.4721(21)                        | [S1] [S2] [S1] [S1] [S2] |
|                                                                                                                              | -10813.4711(24)                        | [S1] [S1] [S2] [S1] [S2] |
|                                                                                                                              | -10813.4717(24)                        | [S1] [S2] [S2] [S1] [S2] |
|                                                                                                                              | -10813.4721(22)                        | [S1] [S1] [S1] [S1] [S1] |
|                                                                                                                              | -10813.4730(22)                        | [S1] [S2] [S1] [S1] [S1] |
|                                                                                                                              | -10813.4717(26)                        | [S1] [S1] [S2] [S1] [S1] |
|                                                                                                                              | -10813.4726(27)                        | [S1] [S2] [S2] [S1] [S1] |
|                                                                                                                              | -10813.4717(20)                        | [S1] [S1] [S1] [S1] [S2] |
|                                                                                                                              | -10813.4726(22)                        | [S1] [S2] [S1] [S1] [S2] |
|                                                                                                                              | -10813.4713(24)                        | [S1] [S1] [S2] [S1] [S2] |
|                                                                                                                              | -10813.4722(25)                        | [S1] [S2] [S2] [S1] [S2] |
| Mean                                                                                                                         | -10813.4721(22) <sup>a</sup>           |                          |

<sup>a</sup> The results listed in the second column are dependent. The numbers in parentheses therefore give the mean uncertainty of the individual values in units of the last digit.

TABLE II. Determination of the  $8s [3/2]_1$  to  $6s [3/2]_2$  wavenumber interval (in  $\text{cm}^{-1}$ ) for the  $^{136}\text{Xe}$  isotope. The first column indicates the sequence of measured transitions used to connect these two states and the arrows point away from (towards) the lower-(higher-)lying energy level. The references in the third column give the sources of the data used in the same order as in the first column (see text for details).

| Connection from $8s [3/2]_1$ to $6s [3/2]_2$ state                                                    | $(E_{6s [3/2]_2} - E_{8s [3/2]_1})/hc$ | Data origin         |
|-------------------------------------------------------------------------------------------------------|----------------------------------------|---------------------|
| $8s [3/2]_1 \leftarrow 6p [5/2]_2 \leftarrow 6s [3/2]_2$                                              | -23864.8833(14)                        | [S1] [S1]           |
|                                                                                                       | -23864.8839(15)                        | [S1] [S2]           |
| $8s [3/2]_1 \leftarrow 6p [3/2]_2 \leftarrow 6s [3/2]_2$                                              | -23864.8835(14)                        | [S1] [S1]           |
|                                                                                                       | -23864.8844(16)                        | [S1] [S2]           |
| $8s [3/2]_1 \leftarrow 6p [1/2]_1 \rightarrow 7s [3/2]_2 \leftarrow 6p [5/2]_2 \leftarrow 6s [3/2]_2$ | -23864.8846(20)                        | [S1] [S1] [S1] [S1] |
|                                                                                                       | -23864.8852(21)                        | [S1] [S1] [S1] [S2] |
| Mean                                                                                                  | -23864.8841(17) <sup>a</sup>           |                     |

<sup>a</sup> The results listed in the second column are dependent. The numbers in parentheses therefore give the mean uncertainty of the individual values in units of the last digit.

TABLE III. Determination of the 6p  $[1/2]_0$  to 6s  $[3/2]_2$  wavenumber interval (in  $\text{cm}^{-1}$ ) for the  $^{136}\text{Xe}$  isotope. The first column indicates the sequence of measured transitions used to connect these two states and the arrows point away from (towards) the lower-lying (higher-lying) energy level. The references in the third column give the sources of the data used in the same order as in the first column (see text for details).

| Connection from 6p $[1/2]_0$ to 6s $[3/2]_2$ state                              | $(E_{6s[3/2]_2} - E_{6p[1/2]_0})/hc$ | Data origin    |
|---------------------------------------------------------------------------------|--------------------------------------|----------------|
| 6p $[1/2]_0 \rightarrow 5d [3/2]_1 \leftarrow 6p [3/2]_1 \leftarrow 6s [3/2]_2$ | -13051.4114(17)                      | [S1] [S1] [S1] |
|                                                                                 | -13051.4118(14)                      | [S2] [S1] [S1] |
|                                                                                 | -13051.4118(21)                      | [S1] [S1] [S2] |
|                                                                                 | -13051.4122(19)                      | [S2] [S1] [S2] |
| 6p $[1/2]_0 \rightarrow 7d [3/2]_1 \leftarrow 6p [3/2]_1 \leftarrow 6s [3/2]_2$ | -13051.4100(17)                      | [S1] [S1] [S1] |
|                                                                                 | -13051.4104(21)                      | [S1] [S1] [S2] |
| 6p $[1/2]_0 \rightarrow 7d [1/2]_1 \leftarrow 6p [3/2]_2 \leftarrow 6s [3/2]_2$ | -13051.4106(17)                      | [S1] [S1] [S1] |
|                                                                                 | -13051.4115(19)                      | [S1] [S1] [S2] |
| 6p $[1/2]_0 \rightarrow 6d [3/2]_1 \leftarrow 6p [5/2]_2 \leftarrow 6s [3/2]_2$ | -13051.4108(17)                      | [S1] [S1] [S1] |
|                                                                                 | -13051.4114(18)                      | [S1] [S1] [S2] |
| 6p $[1/2]_0 \rightarrow 6d [3/2]_1 \leftarrow 6p [3/2]_1 \leftarrow 6s [3/2]_2$ | -13051.4103(17)                      | [S1] [S1] [S1] |
|                                                                                 | -13051.4107(21)                      | [S1] [S1] [S2] |
| Mean                                                                            | -13051.4111(18) <sup>a</sup>         |                |

<sup>a</sup> The results listed in the second column are dependent. The numbers in parentheses therefore give the mean uncertainty of the individual values in units of the last digit.

TABLE IV. Determination of the 8d  $[1/2]_1$  to 6p  $[1/2]_0$  wavenumber interval (in  $\text{cm}^{-1}$ ) for the  $^{136}\text{Xe}$  isotope. The first column indicates the sequence of measured transitions used to connect these two states and the arrows point away from (towards) the lower-lying (higher-lying) energy level. The references in the third column give the sources of the data used in the same order as in the first column (see text for details).

| Connection from 8d $[1/2]_1$ to 6p $[1/2]_0$ state                                                                           | $(E_{6p[1/2]_0} - E_{8d[1/2]_1})/hc$ | Data origin              |
|------------------------------------------------------------------------------------------------------------------------------|--------------------------------------|--------------------------|
| 8d $[1/2]_1 \leftarrow 6p [5/2]_2 \rightarrow 6d [3/2]_1 \leftarrow 6p [1/2]_0$                                              | -14109.0435(17)                      | [S1] [S1] [S1]           |
| 8d $[1/2]_1 \leftarrow 6p [5/2]_2 \leftarrow 6s [3/2]_2 \rightarrow 6p [3/2]_1 \rightarrow 5d [3/2]_1 \leftarrow 6p [1/2]_0$ | -14109.0429(22)                      | [S1] [S1] [S1] [S1] [S1] |
|                                                                                                                              | -14109.0435(23)                      | [S1] [S2] [S1] [S1] [S1] |
|                                                                                                                              | -14109.0425(26)                      | [S1] [S1] [S2] [S1] [S1] |
|                                                                                                                              | -14109.0431(26)                      | [S1] [S2] [S2] [S1] [S1] |
|                                                                                                                              | -14109.0425(20)                      | [S1] [S1] [S1] [S1] [S2] |
|                                                                                                                              | -14109.0431(21)                      | [S1] [S2] [S1] [S1] [S2] |
|                                                                                                                              | -14109.0421(24)                      | [S1] [S1] [S2] [S1] [S2] |
|                                                                                                                              | -14109.0427(24)                      | [S1] [S2] [S2] [S1] [S2] |
| 8d $[1/2]_1 \leftarrow 6p [3/2]_2 \rightarrow 7d [1/2]_1 \leftarrow 6p [1/2]_0$                                              | -14109.0440(17)                      | [S1] [S1] [S1]           |
| 8d $[1/2]_1 \leftarrow 6p [3/2]_2 \leftarrow 6s [3/2]_2 \rightarrow 6p [3/2]_1 \rightarrow 5d [3/2]_1 \leftarrow 6p [1/2]_0$ | -14109.0432(22)                      | [S1] [S1] [S1] [S1] [S1] |
|                                                                                                                              | -14109.0441(24)                      | [S1] [S2] [S1] [S1] [S1] |
|                                                                                                                              | -14109.0428(26)                      | [S1] [S1] [S2] [S1] [S1] |
|                                                                                                                              | -14109.0437(27)                      | [S1] [S2] [S2] [S1] [S1] |
|                                                                                                                              | -14109.0428(20)                      | [S1] [S1] [S1] [S1] [S2] |
|                                                                                                                              | -14109.0437(22)                      | [S1] [S2] [S1] [S1] [S2] |
|                                                                                                                              | -14109.0424(24)                      | [S1] [S1] [S2] [S1] [S2] |
|                                                                                                                              | -14109.0433(25)                      | [S1] [S2] [S2] [S1] [S2] |
| 8d $[1/2]_1 \leftarrow 6p [3/2]_1 \rightarrow 5d [3/2]_1 \leftarrow 6p [1/2]_0$                                              | -14109.0450(17)                      | [S1] [S1] [S1]           |
|                                                                                                                              | -14109.0446(14)                      | [S1] [S1] [S2]           |
| 8d $[1/2]_1 \leftarrow 6p [3/2]_1 \rightarrow 7d [3/2]_1 \leftarrow 6p [1/2]_0$                                              | -14109.0464(17)                      | [S1] [S1] [S1]           |
| 8d $[1/2]_1 \leftarrow 6p [3/2]_1 \rightarrow 6d [3/2]_1 \leftarrow 6p [1/2]_0$                                              | -14109.0461(17)                      | [S1] [S1] [S1]           |
| 8d $[1/2]_1 \leftarrow 6p [1/2]_1 \rightarrow 7d [1/2]_1 \leftarrow 6p [1/2]_0$                                              | -14109.0430(17)                      | [S1] [S1] [S1]           |
| 8d $[1/2]_1 \leftarrow 6p [1/2]_1 \rightarrow 6d [3/2]_1 \leftarrow 6p [1/2]_0$                                              | -14109.0434(17)                      | [S1] [S1] [S1]           |
| 8d $[1/2]_1 \leftarrow 6p [1/2]_1 \rightarrow 7d [3/2]_1 \leftarrow 6p [1/2]_0$                                              | -14109.0427(17)                      | [S1] [S1] [S1]           |
| Mean                                                                                                                         | -14109.0435(21) <sup>a</sup>         |                          |

<sup>a</sup> The results listed in the second column are dependent. The numbers in parentheses therefore give the mean uncertainty of the individual values in units of the last digit.

TABLE V. Determination of the 8d  $[1/2]_1$  to 6s  $[3/2]_2$  wavenumber interval (in  $\text{cm}^{-1}$ ) for the  $^{136}\text{Xe}$  isotope. The first column indicates the sequence of measured transitions used to connect these two states and the arrows point away from (towards) the lower-lying (higher-lying) energy level. The references in the third column give the sources of the data used in the same order as in the first column (see text for details).

| Connection from 8d $[1/2]_1$ to 6s $[3/2]_2$ state                                                    | $(E_{6s[3/2]_2} - E_{8d[1/2]_1})/hc$ | Data origin         |
|-------------------------------------------------------------------------------------------------------|--------------------------------------|---------------------|
| 8d $[1/2]_1 \leftarrow 6p [5/2]_2 \leftarrow 6s [3/2]_2$                                              | -27160.4543(14)                      | [S1] [S1]           |
|                                                                                                       | -27160.4549(15)                      | [S1] [S2]           |
| 8d $[1/2]_1 \leftarrow 6p [3/2]_2 \leftarrow 6s [3/2]_2$                                              | -27160.4546(14)                      | [S1] [S1]           |
|                                                                                                       | -27160.4555(16)                      | [S1] [S2]           |
| 8d $[1/2]_1 \leftarrow 6p [3/2]_1 \leftarrow 6s [3/2]_2$                                              | -27160.4564(14)                      | [S1] [S1]           |
|                                                                                                       | -27160.4568(19)                      | [S1] [S2]           |
| 8d $[1/2]_1 \leftarrow 6p [5/2]_2 \rightarrow 6d [3/2]_1 \leftarrow 6p [3/2]_1 \leftarrow 6s [3/2]_2$ | -27160.4538(20)                      | [S1] [S1] [S1] [S1] |
|                                                                                                       | -27160.4542(24)                      | [S1] [S1] [S1] [S2] |
| 8d $[1/2]_1 \leftarrow 6p [1/2]_1 \rightarrow 7s [3/2]_2 \leftarrow 6p [5/2]_2 \leftarrow 6s [3/2]_2$ | -27160.4551(20)                      | [S1] [S1] [S1] [S1] |
|                                                                                                       | -27160.4557(21)                      | [S1] [S1] [S1] [S2] |
| 8d $[1/2]_1 \leftarrow 6p [1/2]_1 \rightarrow 7d [1/2]_1 \leftarrow 6p [3/2]_2 \leftarrow 6s [3/2]_2$ | -27160.4536(20)                      | [S1] [S1] [S1] [S1] |
|                                                                                                       | -27160.4545(22)                      | [S1] [S1] [S1] [S2] |
| 8d $[1/2]_1 \leftarrow 6p [1/2]_1 \rightarrow 6d [3/2]_1 \leftarrow 6p [3/2]_1 \leftarrow 6s [3/2]_2$ | -27160.4537(20)                      | [S1] [S1] [S1] [S1] |
|                                                                                                       | -27160.4541(24)                      | [S1] [S1] [S1] [S2] |
| 8d $[1/2]_1 \leftarrow 6p [1/2]_1 \rightarrow 7d [3/2]_1 \leftarrow 6p [3/2]_1 \leftarrow 6s [3/2]_2$ | -27160.4527(20)                      | [S1] [S1] [S1] [S1] |
|                                                                                                       | -27160.4531(24)                      | [S1] [S1] [S1] [S2] |
| Mean                                                                                                  | -27160.4546(19) <sup>a</sup>         |                     |

<sup>a</sup> The results listed in the second column are dependent. The numbers in parentheses therefore give the mean uncertainty of the individual values in units of the last digit.

TABLE VI. Determination of the 6s  $[3/2]_2$  to 6s'  $[1/2]_0$  wavenumber interval (in  $\text{cm}^{-1}$ ) for the  $^{136}\text{Xe}$  isotope. The first column indicates the sequence of measured transitions used to connect these two states and the arrows point away from (towards) the lower-(higher-)lying energy level. The references in the third column give the sources of the data used in the same order as in the first column (see text for details).

| Connection from 6s $[3/2]_2$ to 6s' $[1/2]_0$ state         | $(E_{6s[3/2]_2} - E_{6s'[1/2]_0})/hc$ | Data origin |
|-------------------------------------------------------------|---------------------------------------|-------------|
| 6d $[3/2]_2 \rightarrow 6p' [1/2]_1 \leftarrow 6s' [1/2]_0$ | 9129.2214(14)                         | [S1] [S1]   |
| 6d $[3/2]_2 \rightarrow 8p [1/2]_1 \leftarrow 6s' [1/2]_0$  | 9129.2198(14)                         | [S1] [S1]   |
| 6d $[3/2]_2 \rightarrow 4f [3/2]_1 \leftarrow 6s' [1/2]_0$  | 9129.2216(14)                         | [S1] [S1]   |
| 6d $[3/2]_2 \rightarrow 7p [3/2]_1 \leftarrow 6s' [1/2]_0$  | 9129.2215(14)                         | [S1] [S1]   |
| 6d $[3/2]_2 \rightarrow 6p' [3/2]_1 \leftarrow 6s' [1/2]_0$ | 9129.2215(14)                         | [S1] [S1]   |
| 6d $[3/2]_2 \rightarrow 7p [1/2]_1 \leftarrow 6s' [1/2]_0$  | 9129.2209(14)                         | [S1] [S1]   |
| Mean                                                        | 9129.2211(14) <sup>a</sup>            |             |

<sup>a</sup> The results listed in the second column are dependent. The numbers in parentheses therefore give the mean uncertainty of the individual values in units of the last digit.

TABLE VII. Determination of the isotopic shifts  $\Delta E_I^{A,136}/h = (E_I^A - E_I^{136})/h$  of the  $\text{Xe}^+ (5p)^5 2P_{3/2} \leftarrow \text{Xe} (5p)^6 1S_0$  first ionization frequency  $E_I^A/h$  of the main natural isotopes ( $A = 128, 129, 130, 131, 132, 134$ ) of xenon relative to that of the  $^{136}\text{Xe}$  isotope. The first column indicates the sequence of measured frequencies used to determine  $\Delta E_I^{A,136}/h$  and the arrows point away from (towards) the lower-lying (higher-lying) energy level. All values are given in MHz. The references in the last column give the sources of the data used in the same order as in the first column (see text for details).

|                                                                                                                                                                                                                         | $\Delta_{128,136}^{\text{ion}}$ | $\Delta_{129,136}^{\text{ion}}$ | $\Delta_{130,136}^{\text{ion}}$ | $\Delta_{131,136}^{\text{ion}}$ | $\Delta_{132,136}^{\text{ion}}$ | $\Delta_{134,136}^{\text{ion}}$ | Data origin      |      |      |           |
|-------------------------------------------------------------------------------------------------------------------------------------------------------------------------------------------------------------------------|---------------------------------|---------------------------------|---------------------------------|---------------------------------|---------------------------------|---------------------------------|------------------|------|------|-----------|
| $(5p)^6\ ^1S_0 \rightarrow 6p\ [3/2]_2 \leftarrow 6s\ [3/2]_2 \rightarrow \text{Ion. limit}$                                                                                                                            |                                 |                                 |                                 |                                 |                                 |                                 |                  |      |      |           |
| —                                                                                                                                                                                                                       | —                               | -716.6(2.1)                     | -573.3(4.0)                     | -566.1(2.1)                     | -397.3(0.6)                     | -223.3(1.0)                     | [S8]             | [S6] | [S9] |           |
| —                                                                                                                                                                                                                       | —                               | -713.6(7.0)                     | -574.3(6.0)                     | -550.1(6.0)                     | -397.0(4.0)                     | -222.5(3.1)                     | [S8]             | [S5] | [S9] |           |
| —                                                                                                                                                                                                                       | —                               | -720.7(5.3)                     | -576.7(6.7)                     | -555.3(3.7)                     | -402.0(9.1)                     | -219.2(4.6)                     | [S8]             | [S7] | [S9] |           |
| —                                                                                                                                                                                                                       | —                               | -712.4(15.0)                    | -573.7(9.0)                     | -548.9(15.0)                    | -393.9(9.0)                     | -221.4(9.0)                     | [S8]             | [S3] | [S9] |           |
| $(5p)^6\ ^1S_0 \rightarrow 6p\ [1/2]_0 \leftarrow 6s\ [3/2]_1 \rightarrow 6p\ [3/2]_2 \leftarrow 6s\ [3/2]_2 \rightarrow \text{Ion. limit}$                                                                             |                                 |                                 |                                 |                                 |                                 |                                 |                  |      |      |           |
| —                                                                                                                                                                                                                       | —                               | -721.6(9.4)                     | —                               | -568.0(10.3)                    | -403.9(8.4)                     | -224.6(9.9)                     | [ <sup>a</sup> ] | [S7] | [S7] | [S6] [S9] |
| —                                                                                                                                                                                                                       | —                               | -711.4(8.7)                     | —                               | -556.6(8.7)                     | -400.6(7.5)                     | -231.5(10.1)                    | [ <sup>a</sup> ] | [S3] | [S7] | [S6] [S9] |
| —                                                                                                                                                                                                                       | —                               | —                               | —                               | —                               | -401.5(7.4)                     | -226.6(7.3)                     | [ <sup>a</sup> ] | [S7] | [S3] | [S6] [S9] |
| —                                                                                                                                                                                                                       | —                               | —                               | —                               | —                               | -398.2(6.4)                     | -233.5(7.3)                     | [ <sup>a</sup> ] | [S3] | [S3] | [S6] [S9] |
| —                                                                                                                                                                                                                       | —                               | -718.6(11.6)                    | —                               | -552.0(11.7)                    | -403.6(9.3)                     | -223.8(10.3)                    | [ <sup>a</sup> ] | [S7] | [S7] | [S5] [S9] |
| —                                                                                                                                                                                                                       | —                               | -708.4(11.0)                    | —                               | -540.6(10.4)                    | -400.3(8.5)                     | -230.7(10.5)                    | [ <sup>a</sup> ] | [S3] | [S7] | [S5] [S9] |
| —                                                                                                                                                                                                                       | —                               | —                               | —                               | —                               | -401.2(8.4)                     | -225.8(7.8)                     | [ <sup>a</sup> ] | [S7] | [S3] | [S5] [S9] |
| —                                                                                                                                                                                                                       | —                               | —                               | —                               | —                               | -397.9(7.5)                     | -232.7(8.1)                     | [ <sup>a</sup> ] | [S3] | [S3] | [S5] [S9] |
| —                                                                                                                                                                                                                       | —                               | -725.7(10.6)                    | —                               | -557.2(10.7)                    | -408.6(12.4)                    | -220.5(10.9)                    | [ <sup>a</sup> ] | [S7] | [S7] | [S7] [S9] |
| —                                                                                                                                                                                                                       | —                               | -715.4(10.0)                    | —                               | -545.8(9.3)                     | -405.3(11.8)                    | -227.4(11.1)                    | [ <sup>a</sup> ] | [S3] | [S7] | [S7] [S9] |
| —                                                                                                                                                                                                                       | —                               | —                               | —                               | —                               | -406.2(11.7)                    | -222.5(8.6)                     | [ <sup>a</sup> ] | [S7] | [S3] | [S7] [S9] |
| —                                                                                                                                                                                                                       | —                               | —                               | —                               | —                               | -402.9(11.1)                    | -229.4(8.8)                     | [ <sup>a</sup> ] | [S3] | [S3] | [S7] [S9] |
| —                                                                                                                                                                                                                       | —                               | -717.4(17.6)                    | —                               | -550.8(18.1)                    | -400.5(12.3)                    | -222.7(13.3)                    | [ <sup>a</sup> ] | [S7] | [S7] | [S3] [S9] |
| —                                                                                                                                                                                                                       | —                               | -707.2(17.2)                    | —                               | -539.4(17.2)                    | -397.2(11.7)                    | -229.6(13.5)                    | [ <sup>a</sup> ] | [S3] | [S7] | [S3] [S9] |
| —                                                                                                                                                                                                                       | —                               | —                               | —                               | —                               | -398.1(11.6)                    | -224.7(11.5)                    | [ <sup>a</sup> ] | [S7] | [S3] | [S3] [S9] |
| —                                                                                                                                                                                                                       | —                               | —                               | —                               | —                               | -394.8(11.0)                    | -231.6(11.7)                    | [ <sup>a</sup> ] | [S3] | [S3] | [S3] [S9] |
| -770.0(34.5)                                                                                                                                                                                                            | -719.0(9.6)                     | -574.3(25.8)                    | -566.3(10.4)                    | -401.8(8.4)                     | -223.8(9.9)                     |                                 | [S4]             | [S7] | [S7] | [S6] [S9] |
| -775.9(31.6)                                                                                                                                                                                                            | -708.8(8.9)                     | -577.7(24.1)                    | -554.9(8.9)                     | -398.5(7.6)                     | -230.7(10.1)                    |                                 | [S4]             | [S3] | [S7] | [S6] [S9] |
| -768.1(16.2)                                                                                                                                                                                                            | —                               | -571.4(12.6)                    | —                               | -399.4(7.4)                     | -225.8(7.3)                     |                                 | [S4]             | [S7] | [S3] | [S6] [S9] |
| -774.0(8.6)                                                                                                                                                                                                             | —                               | -574.8(8.6)                     | —                               | -396.1(6.5)                     | -232.7(7.6)                     |                                 | [S4]             | [S3] | [S3] | [S6] [S9] |
| -763.5(35.9)                                                                                                                                                                                                            | -716.0(11.7)                    | -575.3(26.2)                    | -550.3(11.8)                    | -401.5(9.3)                     | -223.0(10.3)                    |                                 | [S4]             | [S7] | [S7] | [S5] [S9] |
| -769.4(33.2)                                                                                                                                                                                                            | -705.8(11.1)                    | -578.7(24.5)                    | -538.9(10.5)                    | -398.2(8.6)                     | -229.9(10.5)                    |                                 | [S4]             | [S3] | [S7] | [S5] [S9] |
| -761.6(19.1)                                                                                                                                                                                                            | —                               | -572.4(13.4)                    | —                               | -399.1(8.4)                     | -225.0(7.9)                     |                                 | [S4]             | [S7] | [S3] | [S5] [S9] |
| -767.5(13.2)                                                                                                                                                                                                            | —                               | -575.8(9.7)                     | —                               | -395.8(7.6)                     | -231.9(8.1)                     |                                 | [S4]             | [S3] | [S3] | [S5] [S9] |
| -776.2(35.1)                                                                                                                                                                                                            | -723.1(10.8)                    | -577.7(26.4)                    | -555.5(10.8)                    | -406.5(12.4)                    | -219.7(10.9)                    |                                 | [S4]             | [S7] | [S7] | [S7] [S9] |
| -782.1(32.3)                                                                                                                                                                                                            | -712.9(10.1)                    | -581.1(24.7)                    | -544.1 (9.4)                    | -403.2(11.8)                    | -226.6(11.1)                    |                                 | [S4]             | [S3] | [S7] | [S7] [S9] |
| -774.3(17.5)                                                                                                                                                                                                            | —                               | -574.8(13.7)                    | —                               | -404.1(11.7)                    | -221.7(8.6)                     |                                 | [S4]             | [S7] | [S3] | [S7] [S9] |
| -780.2(10.8)                                                                                                                                                                                                            | —                               | -578.2(10.1)                    | —                               | -400.8(11.1)                    | -228.6(8.8)                     |                                 | [S4]             | [S3] | [S3] | [S7] [S9] |
| -767.8(35.6)                                                                                                                                                                                                            | -714.8(17.7)                    | -574.7(27.1)                    | -549.1(18.1)                    | -398.4(12.3)                    | -221.9(13.4)                    |                                 | [S4]             | [S7] | [S7] | [S3] [S9] |
| -773.7(32.9)                                                                                                                                                                                                            | -704.6(17.3)                    | -578.1(25.4)                    | -537.7(17.3)                    | -395.1(11.8)                    | -228.8(13.5)                    |                                 | [S4]             | [S3] | [S7] | [S3] [S9] |
| -765.9(18.6)                                                                                                                                                                                                            | —                               | -571.8(15.0)                    | —                               | -396.0(11.7)                    | -223.0(11.6)                    |                                 | [S4]             | [S7] | [S3] | [S3] [S9] |
| -771.8(12.5)                                                                                                                                                                                                            | —                               | -575.2(11.8)                    | —                               | -392.7(11.1)                    | -230.8(11.7)                    |                                 | [S4]             | [S3] | [S3] | [S3] [S9] |
| Weighted mean including $\Delta_{128,136}^{\text{ion}}$ $\Delta_{129,136}^{\text{ion}}$ $\Delta_{130,136}^{\text{ion}}$ $\Delta_{131,136}^{\text{ion}}$ $\Delta_{132,136}^{\text{ion}}$ $\Delta_{134,136}^{\text{ion}}$ |                                 |                                 |                                 |                                 |                                 |                                 |                  |      |      |           |
| All data                                                                                                                                                                                                                | -772.3(5.1)                     | -716.2(3.7)                     | -574.6(1.8)                     | -559.3(8.3)                     | -397.6(1.5)                     | -224.0(2.7)                     |                  |      |      |           |
| First transition from [S8]                                                                                                                                                                                              | —                               | -716.8(1.7)                     | -574.2(1.2)                     | -562.3(5.9)                     | -397.3(0.4)                     | -223.1(0.8)                     |                  |      |      |           |
| First transition from [ <sup>a</sup> ]                                                                                                                                                                                  | —                               | -716.2(5.9)                     | —                               | -552.5(8.8)                     | -400.9(3.1)                     | -227.7(3.9)                     |                  |      |      |           |
| First transition from [S4]                                                                                                                                                                                              | -772.3(5.1)                     | -713.6(5.9)                     | -575.2(2.3)                     | -550.8(8.8)                     | -398.7(3.1)                     | -226.9(3.9)                     |                  |      |      |           |

<sup>a</sup> This work.

- 
- [S1] C. J. Humphreys and E. Paul Jr., Interferometric wavelength determination in the first spectrum of  $^{136}\text{Xe}$ , *J. Opt. Soc. Am.* **60**, 1302 (1970).
  - [S2] T. A. Littlefield and M. Rafi, Interferometric wavelength measurements in the infra-red spectrum of isotope xenon 136, *J. Phys. B: At. Mol. Phys.* **7**, 612 (1974).
  - [S3] D. A. Jackson and M.-C. Coulombe, Isotope shifts in the arc spectrum of xenon, *Proc. R. Soc. London A* **338**, 277 (1974).
  - [S4] M. D. Plimmer, P. E. G. Baird, C. J. Foot, D. N. Stacey, J. B. Swan, and G. K. Woodgate, Isotope shift in xenon by Doppler-free two-photon laser spectroscopy, *J. Phys. B: At. Mol. Opt. Phys.* **22**, L241 (1989).
  - [S5] W. Borchers, E. Arnold, W. Neu, R. Neugart, K. Wendt, G. Ulm, and ISOLDE Collaboration, Xenon isotopes far from stability studied by collisional ionization laser spectroscopy, *Phys. Lett. B* **216**, 7 (1989).
  - [S6] G. D'Amico, G. Pesce, and A. Sasso, Isotope-shift and hyperfine-constant measurements of near-infrared xenon transitions in glow discharges and on a metastable  $\text{Xe}(^3P_2)$  beam, *Phys. Rev. A* **60**, 4409 (1999).
  - [S7] M. Suzuki, K. Katoh, and N. Nishimiya, Saturated absorption spectroscopy of Xe using a GaAs semiconductor laser, *Spectrochim. Acta A* **58**, 2519 (2002).
  - [S8] E. Altieri, E. R. Miller, T. Hayamizu, D. J. Jones, K. W. Madison, and T. Momose, High-resolution two-photon spectroscopy of a  $5p^56p \leftarrow 5p^6$  transition of xenon, *Phys. Rev. A* **97**, 012507 (2018).
  - [S9] H. Herburger, E. N. Toutoudaki, U. Hollenstein, and F. Merkt, High-resolution spectroscopy and multichannel quantum-defect-theory analysis of the  $np$  and  $nf$  Rydberg series of Xe below the  $^2P_{3/2}$  ionization threshold, *Phys. Rev. A* **109**, 032816 (2024).
  - [S10] R. D. Knight and L.-g. Wang, One-photon laser spectroscopy of the  $np$  and  $nf$  Rydberg series in xenon, *J. Opt. Soc. Am. B* **2**, 1084 (1985).
  - [S11] F. Brandi, I. Velchev, W. Hogervorst, and W. Ubachs, Vacuum-ultraviolet spectroscopy of Xe: Hyperfine splittings, isotope shifts, and isotope-dependent ionization energies, *Phys. Rev. A* **64**, 032505 (2001).
  - [S12] L. S. Dreissen, C. Roth, E. L. Gründeman, J. J. Krauth, M. Favier, and K. S. E. Eikema, High-Precision Ramsey-Comb Spectroscopy Based on High-Harmonic Generation, *Phys. Rev. Lett.* **123**, 143001 (2019).
  - [S13] L. S. Dreissen, C. Roth, E. L. Gründeman, J. J. Krauth, M. G. J. Favier, and K. S. E. Eikema, Ramsey-comb precision spectroscopy in xenon at vacuum ultraviolet wavelengths produced with high-order harmonic generation, *Phys. Rev. A* **101**, 052509 (2020).
